# Supplementary material for: USB-NeRF: Unrolling Shutter Bundle Adjusted Neural Radiance Fields
Source: arXiv:2310.02687 source file (2024-02-26)
Supplement: Supplementary file 1 [file rebuttal_exp.tex]

\section{Experiments}\label{sec:experiment_rebuttal}
%
%
%
%

\red{\PAR{Response to Reviewer CtJa}}

We thank the reviewer for the acknowledgement of the technical novelty and soundness of our method. We make replies to the questions from the reviewer as follows:

We captured 5 additional sequences using GoPro HERO6 Black, Canon camera (EOS M3), and iPhone 14 Pro, and made more analysis on real-world datasets. All rolling shutter images are captured at the frequency of 30Hz. We find that the captured images with modern cameras still exhibit obvious RS effects if they undergo fast motions, which can easily happen for certain scenarios, e.g. GoPro carried by a flying drone, which is a common set-up for most hobbyists or taking photos on a moving vehicle.

Since it is hardly to capture corresponding GS images, we only make qualitative comparisons on these datasets. Please refer to Figure 10, Figure 11, and Figure 12 in Appendix A.3 of the main paper for the experimental results on real-world datasets.
%
The experimental results demonstrate that: 1) both NeRF and BARF fail to correct the RS effect distortion; 2) both NeRF and BARF produce significant artifacts if the camera motion is not in a constant direction (e.g. the camera is moving forward and then backward); 3) our method corrects the RS effect distortion with no artifact; 4) it is still valuable to model RS effect for certain scenarios with modern cameras.

%NeRF would fail in some scenes, as images with RS effect will cause pose estimation inaccuracy and they do not satisfy multi-view consistency. Although BARF could also optimize pose, it could not find the accurate pose to satisfy geometric constraints without modelling rolling shutter effect, thus causing blur in some views. While our method could synthesize corrected GS images of good quality by modelling physical rolling shutter image formation process.

\red{\PAR{Response to Reviewer wLRe}}

We thank the reviewer for the effort spent in reviewing our paper and the acknowledgement of the improved performance with rolling shutter modeling. We make replies to the questions from the reviewer as follows:

\PAR{Q1: I am not fully convinced that using rolling shutter camera is an effective way to capture a NeRF model.}

A1: As the comment from reviewer CtJa, most consumer products (e.g. GoPro camera, DSLR camera and iPhone 14 Pro) still use rolling shutter cameras for photo capture and video recording nowadays. Since we usually capture images in a slow motion, the RS effect is often negligible. However, there are still obvious RS distortions for certain cases if the camera undergoes fast motion, e.g. recording videos with a GoPro camera carried by a flying drone, which is a common setup for most hobbyists. Therefore, it is valuable to model RS effect for NeRF reconstruction. 

\PAR{Q2: The proposed method is a simple two-step approach, which lacks novelty.}

A2: Our method \textbf{is not a simple two-step approach}, which conducts rolling shutter correction first and then run normal NeRF reconstruction. Instead, our method \textbf{is a single-step method}. In particular, we integrate the RS image formation model into the framework of NeRF, and use RS images to directly reconstruct the true underlying 3D scene representation with NeRF, which has not been done by any prior work. Once the model is trained, corrected global shutter images can be rendered from NeRF to achieve rolling shutter effect correction.

%For weakness 1, rolling shutter cameras are widely used in the consumer market because of their lower price. Smartphones also use rolling shutter cameras (Please refer to Figure 12 for rolling shutter images we captured through iPhone 14 Pro). Now most NeRF-based methods require inputs without RS effect, motion blur, etc. However perfect images are difficult to get in the real world. If we want to use real-world datasets for scene reconstruction, the neglect of the rolling shutter effect will sometimes cause huge performance degradation of NeRF due to the inaccurate pose estimation and geometric inconsistency. We conduct more experiments on real-world datasets to demonstrate the necessity of taking rolling shutter effect correction into consideration. Please refer to Figure 10, 11, 12 of Appendix A.3 in the modified main paper for more results on real-world datasets.
%
%For weakness 2, our method is not a two-stage method. We use cubic B-Spline for trajectory representation and NeRF as scene representation, and make joint optimization of NeRF and trajectory to simultaneously realize rolling shutter effect correction and scene reconstruction.

\PAR{Q3: No examples contain moving objects.}
A3: Our method is currently not modeled to work for dynamic environments. However, our method is the first to train NeRF with rolling shutter images of static environment. We propose to divide the solution into two steps: handle static environment first, and leave the solution for dynamic environments as our next work. The capability to handle static environments would already be useful for many application scenarios. On the other hand, to handle dynamic environments with NeRF itself is also an on-going research.

\PAR{Q4: I am not convinced that a user would purposely move the camera in high speed and it is an uncommon scenario to have such rolling shutter effects unless they are captured on purpose.}

The rolling shutter effect is not negligible for certain scenarios and not purposely to have it. For example, to reconstruct a 3D scene with a GoPro camera carried by a fast flying drone. It would affect the users experience to instruct them to fly the quad-copter slowly, due to our software cannot handle RS distortion. It is also not practical to ask them to replace their GoPro camera with a more expensive global shutter camera, which could also be bulky for the drone to carry.

If we could have the solution without requiring any changes for the end consumers, we think it would still be beneficial to have it. 

\PAR{Q5: I am puzzle why such simple 2-step approach do not work on this application scenario? Although you have provided comparisons with RS corrections based on deep learning, there are many traditional rolling shutter correction methods that can be applied in this application scenario and they do not require training data. In particular...}

We will reply from following perspectives:

1) A simple 2-step approach would heavily rely on the performance of the RS correction step. Instead of doing this, we did not do explicit RS correction and integrate the image formation model into NeRF, such that NeRF can be learned from RS images directly; The experimental results demonstrate our method can deliver good performance;

2) We do compare against such 2-step approach in our paper, as the reviewer also agrees, except that we do not compare against traditional approach + NeRF; Due to the generalization performance, deep learning based 2-step approach does not work well as what we demonstrate in our experiments;

3) The three traditional methods suggested by the reviewer have no implementation released to the public. Even though, we implemented the ``Rolling Shutter Bundle Adjustment, CVPR 2012'' paper by ourself for comparisons. The experimental results are presented in Table 3, Table 8, Table 9 and Table 10. The shortcut ``RSBA'' is for this work and we explained it in the ``Evaluation metrics'' section on page 7;

We also implement another more recent traditional approach ``NW-RSBA, CVPR 2023'' for better evaluations; 

4) The method from ``Rolling Shutter Bundle Adjustment, CVPR 2012'' does not support rolling shutter correction. It is designed to do sparse bundle adjustment with rolling shutter images, and there is no dense rolling shutter correction involved;

5) The method from ``Global Optimization of Object Pose and Motion from a Single Rolling Shutter Image with Automatic 2D-3D Matching, ECCV 2012'' does not support rolling shutter correction either. It is designed to estimate the pose of a moving object relative to the camera. There is no dense rolling shutter correction involved;

6) The method from ``Calibration-free rolling shutter removal, ICCP 2012'' does consider rolling shutter correction. However, they exploit homography to formulate the problem, which would fail if the scene is composed of layers with large differences in depth. In contrary, our method does not have this limitation, and can handle general scenarios, as the results in Figure 10 demonstrate. 

By considering all these factors, we only re-implement two traditional methods "RSBA, CVPR 2012'' and "NW-RSBA, CVPR 2023'' for evaluations. Traditional methods, such as "Calibration-free rolling shutter removal, ICCP 2012'' usually have strong assumptions and cannot deliver good RS correction results for general scenarios. We therefore did not re-implement and compare against them for the 2-step approaches. Our method does not have such limitations.

\PAR{Q6: Note that you have also cited the CVPR 2012 paper (Hedborget al.,2012) and claimed that their model does not work. However, there is no such comparison in the paper.}

We do have this comparison in the paper, the results are presented in Table 3, Table 8, Table 9 and Table 10. The ``RSBA'' shortcut represent the paper and we explained it in the ``Evaluation metrics'' section on page 7. Since RSBA is used to estimate the camera pose and reconstruct 3D points (i.e. Sparse bundle adjustment), we therefore only compare against it in terms of the pose accuracy.

\PAR{Q7: it is disappointed that the paper does not done enough in literature review in rolling shutter correction, and many methods in rolling shutter correction are ignored in the comparisons.} 

We will include more related works. Since there are many prior methods, we are unable to include every related paper, and only present the representative methods that are most related to ours, as presented in the related work section on Page 3.

Based on previous responses, we do compare against prior rolling shutter related methods, even though they do not have their implementations released and we implemented them by ourselves for better evaluations. For the traditional method "Calibration-free rolling shutter removal, ICCP 2012'', we did not re-implement and compare against it since we can already see the advantages of our method over theirs, based on the limitations of their formulation.


\PAR{Providing those clarifications, we sincerely wish and thank the reviewer could re-consider the final rating.}


We thank the reviewer for the prompt feedback and interaction with us. We make replies to the questions from the reviewer as follows. 

\PAR{Q1: Instead, I was questioning the motivations and the necessity of using a rolling shutter camera with fast camera motion to capture a static scene. The rebuttal claimed that GoPro carried by a flying drone is one of the target scenario, but none of the examples were captured under this setting. Again, if it is a static scene, and the user has full controls on capturing device and speed, I do not see a convincing reason to capture a scene with a fast moving rolling shutter camera.}

Our responses are in following two perspectives:

1) It is currently impractical for us to purchase a drone with a GoPro camera to capture the data due to the available time left. However, we tried to simulate the setting as much as possible. For example, the results presented in Figure 11 are captured on a moving tram with a GoPro HERO6. There is no much difference to carry the GoPro camera with a tram or a drone. Furthermore, we also cannot control the speed of a public tram, so it is not on purposely captured either. 

We can do ask them to control the flying speed of the camera, however, it affects the user experience to instruct them "you have to fly slowly due to the RS effect". If they are hobbyists and want to simply do NeRF reconstruction using a video captured during their fun flight (in which they usually aim for fast flight just for fun), they would not choose to control the speed and would choose to throw away the software and choose the one which could satisfy them. 

We simply choose the "GoPro carried by a Drone" as an example. There are also many other example scenarios. For example, the video capture on a moving tram/bus. If we can choose to have this possibility to have a RS NeRF to better handle these scenarios, we think there is no harm to have it.

%2) Another interesting application scenarios is to reconstruct NeRF with images of Google Street View. Google Street View has a repository of billions of 2D images captured with rolling-shutter camera rigs along vehicle trajectories. We also have the simulated data as presented in both Figure 11 and Figure 12. The settings are almost the same, i.e. a moving rolling shutter camera in the city scenario.

2) If the reviewer still disagrees with the above scenarios on the motivation to do NeRF with a rolling shutter camera, our method can also be considered as a dense bundle adjustment method (with NeRF as the underlying 3D representation), which also delivers better performance than prior state-of-the-art methods on rolling shutter aware bundle adjustment, i.e. RSBA-CVPR-2012 and NW-RSBA-CVPR-2023 methods. We also choose to use a public TUM-RS dataset for evaluation to avoid the suspect of using overfitted synthetic datasets. In reality, the trajectories used to create our synthetic datasets are also real trajectories adopted from the ETH3D dataset. It is not on purposely created trajectories.

\PAR{Q2: Regarding whether it's one-step/two-step approach... I believe there is difference when the rolling shutter effects are severe, but the differences would be subtle if the rolling shutter effects are minor. Again, it goes back to the motivation why one has to use fast moving rolling shutter camera to capture a 3D static scene."}

1) To recover high-fidelity high frame-rate global shutter video is based on that the NeRF is already trained with RS images, not the vice verse. It is another advantage of our method over prior one. 

2) Based on the response, I think the reviewer is now convinced that two-step approach would not work well for images with large RS effects.

3) For learning based RS correction method, the difficulty to deliver consistent high-quality global shutter images are not merely caused by the large RS effects. It is mainly caused by the poor generalization performance. Even the RS effect is not large, they might still not be able to generalize well on images from a different distribution domain. Traditional methods usually require strong assumptions for the ease of formulation, it is also fragile to deliver consistent high-quality global shutter images once the assumption is violated. 

4) Furthermore, the dataset that we used for evaluation also does not exhibit very large RS effect. For example, the images presented in Figure 1 of the paper have similar level of RS effects, as what we captured on a city tram, which does not move that fast usually. The experimental results also demonstrate that two-stage approach performs worse than our method, even with these minor realistic RS effects.

5) To do NeRF reconstruction with captured video on a moving city tram/bus, is also a potential real application scenario, which is not on purposely captured either.

If we could have a robust non-fragile method to be able to handle different levels of RS effect in one-go, it would be beneficial to have it. Furthermore, our formulation is also novel and has no generalization problem. 



%3) Both current traditional and deep-learning based methods are unable to deliver high quality global shutter images consistently. If the quality of the recovered global shutter images are not good, it is hard to reconstruct NeRF in high quality. This is the drawback of the two-step approach. It makes the whole pipeline fragile to rely on the rolling shutter correction step.
%
%
%Currently, it is impossible/hardly to recover high frame-rate global shutter video from RS images without NeRF, and then do NeRF reconstruction. 


\PAR{Q3: I asked for the additional comparisons because the major technical challenge in this problem setting is the rolling shutter correction, and the methods you have compared are not targeted for the same application scenario...Of course, if we only look at the quantitative number, one can easily get a better score using synthetic examples since the camera path can be generated to overfit one model over the others...}

1) Our method has two main purposes: a) to do rolling shutter correction under the NeRF framework; b) to do dense bundle adjustment for more accurate pose estimation;

2) Regarding rolling shutter correction, we have compared against prior state-of-the-art deep learning (i.e. DSUN, SUNet, RSSR and CVR) and traditional methods (i.e. DiffSfM-ICCV-2017). Regarding bundle adjustment, we also have compared against prior SOTA methods, i.e. RSBA-CVPR-2012 and NW-RSBA-CVPR-2023. Furthermore, we also compared against NeRF and BARF. 

We could not agree with the reviewer that the methods we have compared are not targeted for the same application scenarios.

3) We also did not use synthetic datasets for the comparisons solely. We also exploit public real dataset from TUM-RS for comparisons on both pose estimation and rolling shutter correction. Furthermore, we also captured additional real dataset, i.e. on a tram/bus with normal moving speed, for qualitative rolling shutter correction experiments. It is also a potential application scenario of our method, i.e. not on purposely captured scenario. These experimental results demonstrate that our method delivers better performance than prior work.

%Our method does have similarity in using cubic-spline or linear interpolation with RSBA-CVPR2012. However, there is another key difference between them, which is that RSBA-CVPR2012 relies on sparse keypoints while our method exploits the full image for optimization with photometric error. Furthermore, the underlying 3D representation is also different, i.e. RSBA-2012 exploits sparse point cloud, while ours exploit a neural network for the representation. We do observe that RSBA has slightly better performance than ours in terms of the ATE metric in Table 8 (on real dataset), however, ours delivers consistent good performance, which results in average better performance. 


\red{\PAR{Response to Reviewer UbiP}}

We thank the reviewer for the acknowledgement of the effectiveness of our method and the paper writing quality. We make replies to the questions from the reviewer as follows:


\PAR{Q1: There is a lack of baseline methods for rolling shutter NeRF.}

A1: Since our method is the first NeRF-based method to model the rolling shutter effect, we are unable to conduct the experiment to compare against prior rolling shutter NeRF.

\PAR{Q2: No rotation errors are provided and the unit of ATE is unclear.}

A2: Yes, the ATE metric is mainly for absolute translation error and the unit is in meters. We have added the unit explanation in the table caption of the main paper to make it clearer.

We re-computed the rotation error with the RPE metric (relative pose error) for rotation. The unit is in ``degrees per frame'' (i.e. $\Delta =1$). The results for both synthetic and real datasets are presented in the following table. Due to the space limit, we only report the average metrics here and the details for each sequence can refer to both Table 9 and Table 10 of the main paper. It demonstrates USB-NeRF also has a better rotation estimation accuracy than prior methods. 

\begin{table}[th]
	\begin{center}
%		\vspace{-1em}
		\captionsetup {font={small,stretch=0.5}}
		\caption{{\textbf{Quantitative comparisons on both synthetic and real datasets in terms of the Relative Pose Error for rotation part (\textdegree / frame).}}}
		\label{rpe_rot}
		\vspace{-0.5em}
		%	\setlength\tabcolsep{2pt}
		\scriptsize
		\setlength{\tabcolsep}{2.5mm}
		\setlength{\belowcaptionskip}{-10pt}
		\resizebox{\linewidth}{!}{
			\begin{tabular}{c|c c c c c c}
				\toprule
				\makebox[0.08\textwidth][c]{} & \makebox[0.08\textwidth][c]{\scriptsize COLMAP} & \makebox[0.08\textwidth][c]{\scriptsize BARF} & \makebox[0.08\textwidth][c]{\scriptsize RSBA} & \makebox[0.08\textwidth][c]{\scriptsize NW-RSBA} & \makebox[0.08\textwidth][c]{\scriptsize USB-NeRF-linear} &\makebox[0.08\textwidth][c]{\scriptsize USB-NeRF-cubic} \\
				%			&{\scriptsize \qquad COLMAP \qquad} &{\scriptsize BARF} &{\scriptsize \qquad RSBA \qquad} & {\scriptsize NW-RSBA} & {\scriptsize \qquad USB-NeRF-linear \qquad} & {\scriptsize \qquad USB-NeRF-cubic \qquad} \\
				\midrule
				
                Synthetic & 2.367$\pm$ 1.348 & 8.386$\pm$ 5.119 & 5.179$\pm$ 2.627 & 2.090$\pm$ 1.492 & 0.446$\pm$ 0.337 & \bf 0.307$\pm$ 0.140 \\

				\midrule
				TUM-RS  & 0.393 $\pm$ 0.218 & 0.429 $\pm$ 0.430 & 2.095 $\pm$ 2.607 & 8.379 $\pm$ 9.928 & 0.283 $\pm$ 0.285 & \bf 0.227 $\pm$ 0.246 \\
				\bottomrule
			\end{tabular}
		}
	\end{center}
\end{table}

\PAR{Q3: The cubic B-Splines interpolation is suitable for complex camera trajectories, however, it can be worse than the linear interpolation method when the camera moves at a constant velocity.}

A3: Cubic B-Splines interpolation is indeed a bit worse than the linear interpolation method when the camera moves at a constant velocity, from the results of Table 1 in the paper. The PSNR metric becomes 0.25 dB worse, which we think is still tolerable.   

\PAR{Q4: BARF looks much worse than NeRF in Fig. 6.}

A4: Thank you for pointing out. We are sorry that we put a wrong figure of BARF in Fig. 6. We corrected it in the main paper now. However, we find that BARF still performs a bit worse than NeRF on the \textit{White Room} sequence. The main reason is that we need to optimize the camera poses of BARF for novel view synthesis experiment, to align the novel view image against the trained scene representation for evaluation. Therefore, the camera pose might converge to a wrong solution sometime if both the learned 3D representation and images are distorted. In contrary, NeRF does not require this since they fix the camera poses which are estimated from COLMAP. 

\PAR{Q5: Can we have a simplified stronger baseline via BARF by splitting the image into R row blocks?}

A5: We conduct this interesting experiment with BARF. In particular, we split every image into both 3 blocks (160 lines per block), and optimize camera pose of each block separately via BARF. We also repeat the experiment with 5 blocks (96 lines per block). The experimental results are presented in following Table on synthetic datasets. It demonstrates that it can have improved performance on some sequences, but could also be worse for others. We think there are two possible reasons: 1) divide the whole image into chunks could indeed help since it suppress the distortions. However, each chunk could still have considerable distortion if the total number of chunks is small, which would affect the performance; 2) divide the whole image into too many chunks would lead to insufficient information of each chunk for individual pose optimization, which would also affect the final performance. Therefore, it would beneficial to model the RS effect into NeRF for better performance. 

\begin{table}[th]
	\begin{center}
		\captionsetup {font={small,stretch=0.5}}
		\caption{{\textbf{Quantitative comparisons on the synthetic datasets in terms of rolling shutter effect removal.}}}
		\label{table_our_syn_barf*_1}
		\vspace{-0.5em}
		\setlength\tabcolsep{2.7pt}
		\setlength{\belowcaptionskip}{-12pt}
		%    \normalsize
		\scriptsize
		\resizebox{\linewidth}{!}{
			\begin{tabular}{c|ccc|ccc|ccc|ccc}
				\toprule
				&  \multicolumn{3}{|c}{Blue Room}  &  \multicolumn{3}{|c}{Living Room}  &  \multicolumn{3}{|c}{White Room} &  \multicolumn{3}{|c}{Avg.}\\
				& PSNR$\uparrow$ & SSIM$\uparrow$ & LPIPS$\downarrow$ & PSNR$\uparrow$ & SSIM$\uparrow$ & LPIPS$\downarrow$ & PSNR$\uparrow$ & SSIM$\uparrow$ & LPIPS$\downarrow$ & PSNR$\uparrow$ & SSIM$\uparrow$ & LPIPS$\downarrow$\\
				\midrule
				BARF \citep{lin2021barf} &19.14 &0.576 &0.3446 & \underline{21.48} &0.690 &0.3341 &18.43 &0.545 &0.3837 &19.68 & 0.604 & 0.3541\\
				
				BARF*(3 blocks) \citep{lin2021barf} & 19.65 & 0.621 & 0.3552 & 19.74 & 0.682 & 0.3565 & 18.47 & 0.532 & 0.3546 & 19.29 & 0.611 & 0.355 \\
				
				BARF*(5 blocks) \citep{lin2021barf} &\underline{20.12} & 0.634 & 0.2429 &17.97 & 0.650 & 0.4310 & \underline{19.04} & 0.557 & 0.3354 &19.04 & 0.614 & 0.3364 \\
				
				\specialrule{0.08em}{1pt}{1pt}
				USB-NeRF (ours) &{\bf 31.85} &{\bf 0.909} &{\bf 0.0573} &{\bf 34.89} &{\bf 0.939} &{\bf 0.0415} &{\bf 30.57} &{\bf 0.892} &{\bf 0.0576} & \bf 32.44 & \bf 0.914 & \bf 0.0521 \\
				\specialrule{0.08em}{1pt}{1pt}
			\end{tabular}
		}
		\vspace{-0.5em}
	\end{center}
\end{table}

%For question 2, we add this experiment and put the results in the following table. We divide every image into 3 blocks (160 lines per block) and 5 blocks (96 lines per block) and optimize camera poses of all blocks through BARF.  \tabnref{table_our_syn_barf*_1} and \tabnref{table_our_syn_barf*_2} demonstrate the results of BARF* \citep{lin2021barf}. After the division of images into several blocks, the performance of BARF on some datasets is even worse. Because the information of every block is less than the information of one image, it is not enough to constrain the registration of BARF. The performance of BARF* is better than vanilla BARF only on Blue Room, White Room, and Adornment, because scenes of these 3 datasets are complex enough to provide sufficient information in all divided blocks to constrain the registration of BARF.

\red{\PAR{Response to Reviwer Xdqv}}

We thank the reviewer for the acknowledgement of the good performance of our method and the effort spent in reviewing our paper. We make replies to the questions from the reviewer as follows:


\PAR{Q1: The contribution and the novelty are limited. The effect of the rolling shutter is well-known in 3D vision community, and many works have been trying to solve it in the past years. The proposed methods only contain the basic concept of modeling a rolling shutter.}

A1: Although rolling shutter effect correction has been researched for many years, prior methods still face challenges to solve it. In contrary, we are the first to formulate the problem under the framework of NeRF and deliver very promising results for the problem. 

%
\PAR{Q2: It seems like the proposed method uses the specific motion model of the camera. It might prevent the proposed method from working on the global shutter dataset(no experiment to prove it) and another dataset that cannot be modeled in bicubic motion(no experiment to prove it).}

A2-1: We conduct experiments with global shutter dataset to prove that our formulation could also work for global shutter images. We exploit three public datasets for NeRF with global shutter images. The results are presented in the following table. It demonstrates that our formulation has comparable performance as prior state-of-the-art methods on global shutter dataset. Note that those methods cannot work on RS dataset as ours.  

\begin{table}[th]
	\begin{center}
		\captionsetup {font={small,stretch=0.5}}
		\caption{{\textbf{Quantitative comparisons on the real-world global shutter datasets LLFF \citep{mildenhall2019llff}}}}
		\label{table_llff_gs}
		\vspace{-0.5em}
		\setlength\tabcolsep{2.7pt}
		\setlength{\belowcaptionskip}{-12pt}
		%    \normalsize
		\scriptsize
		\resizebox{\linewidth}{!}{
			\begin{tabular}{c|ccc|ccc|ccc|ccc}
				\toprule
				&  \multicolumn{3}{|c}{fern}  &  \multicolumn{3}{|c}{flower}  &  \multicolumn{3}{|c}{fortress} &  \multicolumn{3}{|c}{Avg.}\\
				& PSNR$\uparrow$ & SSIM$\uparrow$ & LPIPS$\downarrow$ & PSNR$\uparrow$ & SSIM$\uparrow$ & LPIPS$\downarrow$ & PSNR$\uparrow$ & SSIM$\uparrow$ & LPIPS$\downarrow$ & PSNR$\uparrow$ & SSIM$\uparrow$ & LPIPS$\downarrow$\\
				\midrule
				
				NeRF \citep{mildenhall2020nerf}  & 26.12 & 0.825 & \bf 0.0833 & \bf 30.79 & \bf 0.904 & \bf 0.0218 & 22.29 & \bf 0.836 & \bf 0.0791 & \bf 26.40  & \bf 0.855  & \bf 0.0614  \\
				BARF \citep{lin2021barf} & 25.24 & 0.775 & 0.1953 & 29.54 & 0.846 & 0.0609 & \bf 22.96 & 0.740 & 0.1732 & 25.91  & 0.787  & 0.1431  \\
				USB-NeRF & \bf 26.31 & \bf 0.830 & 0.0863 & 29.51 & 0.836 & 0.0625 & 22.57 & 0.813 & 0.1051 & 26.13  & 0.827  & 0.0846  \\
				
				\specialrule{0.08em}{1pt}{1pt}
			\end{tabular}
		}
		\vspace{-0.5em}
	\end{center}
\end{table}

A2-2: We agree that the cubic B-Spline motion model would not work well for certain very specific motions, such as highly non-linear motions. However, we think cubic B-Spline could handle most real world application scenarios, in which the camera motions are usually smooth.

%For weakness 2, when synthesizing rolling shutter images, we adopt the real motion trajectories from ETH3D. We also made experiments on the real-world dataset TUM-RS and our own captured datasets. The motion of our datasets does not supply some specific cubic motion pattern. Meanwhile, Cubic B-spline is a third-degree polynomial interpolation and could model most motion in the real world, only very little motion can not be modeled. As for our our method's performance on global shutter datasets, we add quantitative comparisons with NeRF, BARF on public real-world global shutter datasets nerf-llff for novel view synthesis and present results in \tabnref{table_llff_gs}. We use the last 10\% of images for evaluation on all 3 datasets. Our method achieves comparable performance with NeRF, BARF on all datasets.

\PAR{Q3: The proposed method requires COLMAP to provide an initial camera pose, which is only mentioned in the footnote.}

A3: We indeed also mentioned it in the ``Implementation and training details'' of the paper. Due to space limit, we put it into our Appendix, i.e. A1, as most prior papers did. Furthermore, using COLMAP to compute an initial pose estimation would make the training more stable, which is also a common practice by most prior works. We do not think it would be a limitation. For certain scenarios, we could also relax the requirement of COLMAP, e.g. to integrate our method into a RS visual odometry pipeline, in which the motion tracker could provide a good initial pose estimation.

\PAR{Q4: A Possible Direction for improvement is to regard the camera motion model as the parameters in the Nerf model and solve it during optimization. To this end, the proposed method can be more general to handle global and rolling shutter datasets. It will be a benefit for the community further.}

A4: Our newly conducted experiments in A2-1 demonstrate that our method is already able to handle global shutter camera as a special case of RS camera. We do agree that integrate camera motion model as part of the NeRF model, could be a possible direction for further improvement. 

\PAR{Q5: To sum up, due to the abovementioned concerns, I cannot give a positive rating to the proposed method in the current version.} 

A5: Providing those newly conducted experiments and explanations, we sincerely thank and wish the reviewer to reconsider the final rating. 


%
% 
% 
% 
%\begin{table}[!ht]
%	\begin{center}
%		\captionsetup {font={small,stretch=0.5}}
%		\caption{{\textbf{Quantitative comparisons on the synthetic datasets in terms of rolling shutter effect removal.}}}
%		\label{table_our_syn_barf*_2}
%		\setlength\tabcolsep{2.7pt}
%		\setlength{\belowcaptionskip}{-12pt}
%		%	\normalsize
%		\scriptsize
%		\resizebox{\linewidth}{!}{
%			\begin{tabular}{c|ccc|ccc|ccc|ccc}
%				\toprule
%				&  \multicolumn{3}{c}{Adornment}  &  \multicolumn{3}{|c}{Factory}  &  \multicolumn{3}{|c}{Tanabata} & \multicolumn{3}{|c}{Avg.}\\
%				& PSNR$\uparrow$ & SSIM$\uparrow$ & LPIPS$\downarrow$ & PSNR$\uparrow$ & SSIM$\uparrow$ & LPIPS$\downarrow$ & PSNR$\uparrow$ & SSIM$\uparrow$ & LPIPS$\downarrow$ & PSNR$\uparrow$ & SSIM$\uparrow$ & LPIPS$\downarrow$\\
%				\midrule
%				BARF \citep{lin2021barf} &17.46 &0.485 &0.5614 & \underline{17.94} &0.459 &0.4361 & \underline{15.28} &0.351 &0.6742 &16.89 & 0.432 & 0.5573 \\
%
%                BARF*(3 blocks) \citep{lin2021barf} & 17.52 & 0.478 & 0.4866 & 17.25 & 0.450 & 0.3764 & 12.12 & 0.308 & 0.6440 & 15.63 & 0.412 & 0.5023 \\
%    
%                BARF*(5 blocks) \citep{lin2021barf} & \underline{17.77} & 0.492 & 0.4554 &17.47 & 0.459 & 0.3636 &12.02 & 0.304 & 0.6528 &15.76 & 0.418 & 0.4906 \\
%                
%				\specialrule{0.08em}{1pt}{1pt}
%				USB-NeRF (ours) &{\bf 29.97} &{\bf 0.876} &{\bf 0.0892} &{\bf 32.67} &{\bf 0.898} &{\bf 0.0819} &{\bf 23.84} &{\bf 0.750} &{\bf 0.1947} & \bf 28.83 & \bf 0.841 & \bf 0.1220 \\	
%				\specialrule{0.08em}{1pt}{1pt}
%			\end{tabular}
%		}
%	\end{center}
%\end{table}



% \begin{table}[t]
% 	\begin{center}
% 		\captionsetup {font={small,stretch=0.5}}
% 		\caption{{\textbf{Quantitative comparisons on the synthetic global shutter datasets}}}
% 		\label{table_syn_gs}
% 		\vspace{-0.5em}
% 		\setlength\tabcolsep{2.7pt}
% 		\setlength{\belowcaptionskip}{-12pt}
% 		%    \normalsize
% 		\scriptsize
% 		\resizebox{\linewidth}{!}{
% 			\begin{tabular}{c|ccc|ccc|ccc|ccc}
% 				\toprule
% 				&  \multicolumn{3}{|c}{Blue Room}  &  \multicolumn{3}{|c}{Living Room}  &  \multicolumn{3}{|c}{White Room} &  \multicolumn{3}{|c}{Avg.}\\
% 				& PSNR$\uparrow$ & SSIM$\uparrow$ & LPIPS$\downarrow$ & PSNR$\uparrow$ & SSIM$\uparrow$ & LPIPS$\downarrow$ & PSNR$\uparrow$ & SSIM$\uparrow$ & LPIPS$\downarrow$ & PSNR$\uparrow$ & SSIM$\uparrow$ & LPIPS$\downarrow$\\
% 				\midrule

%                 NeRF \citep{mildenhall2020nerf} &24.06 & 0.708 & 0.2658 & 33.30 & 0.943 & 0.0421 & 14.69 & 0.378 & 0.6259 & 24.02 & 0.677 & 0.3113 \\
%                 BARF \citep{lin2021barf}  & 23.85 & 0.711 & 0.2448 & 27.31 & 0.826 & 0.1884 & 13.93 & 0.444 & 0.7146 & 21.70 & 0.660 & 0.3826 \\
%                 \specialrule{0.08em}{1pt}{1pt}
%                 USB-NeRF & 26.47 & 0.815 & 0.1011 & 33.19 & 0.935 & 0.0452 & 29.74 & 0.907 & 0.0496 & 29.80 & 0.886 & 0.0653 \\
% 				\specialrule{0.08em}{1pt}{1pt}
% 			\end{tabular}
% 		}
% 		\vspace{-0.5em}
% 	\end{center}
% \end{table}

% \begin{table}[t]
% 	\begin{center}
% 		\captionsetup {font={small,stretch=0.5}}
% 		\caption{{\textbf{Quantitative comparisons on the real-world global shutter datasets LLFF \citep{mildenhall2019llff}}}}
% 		\label{table_llff_gs}
% 		\vspace{-0.5em}
% 		\setlength\tabcolsep{2.7pt}
% 		\setlength{\belowcaptionskip}{-12pt}
% 		%    \normalsize
% 		\scriptsize
% 		\resizebox{\linewidth}{!}{
% 			\begin{tabular}{c|ccc|ccc|ccc|ccc}
% 				\toprule
% 				&  \multicolumn{3}{|c}{fern}  &  \multicolumn{3}{|c}{flower}  &  \multicolumn{3}{|c}{fortress} &  \multicolumn{3}{|c}{horns}\\
% 				& PSNR$\uparrow$ & SSIM$\uparrow$ & LPIPS$\downarrow$ & PSNR$\uparrow$ & SSIM$\uparrow$ & LPIPS$\downarrow$ & PSNR$\uparrow$ & SSIM$\uparrow$ & LPIPS$\downarrow$ & PSNR$\uparrow$ & SSIM$\uparrow$ & LPIPS$\downarrow$\\
% 				\midrule
%                 NeRF \citep{mildenhall2020nerf} & 26.12 & 0.825 & 0.0833 & 27.25 & 0.853 & 0.0550 & 30.79 & 0.904 & 0.0218 & 22.29 & 0.836 & 0.0791 \\
%                 BARF \citep{lin2021barf} & 25.24 & 0.775 & 0.1953 & 20.64 & 0.562 & 0.2268 & 29.54 & 0.846 & 0.0609 & 22.96 & 0.740 & 0.1732 \\
%                 \specialrule{0.08em}{1pt}{1pt}
%                 USB-NeRF & 26.31 & 0.830 & 0.0863 & 26.96 & 0.835 & 0.0657 & 29.51 & 0.836 & 0.0625 & 22.57 & 0.813 & 0.1051 \\

% 				\specialrule{0.08em}{1pt}{1pt}
% 			\end{tabular}
% 		}
% 		\vspace{-0.5em}
% 	\end{center}
% \end{table}

%\begin{table}[t]
%	\begin{center}
%		\captionsetup {font={small,stretch=0.5}}
%		\caption{{\textbf{Quantitative comparisons on synthetic datasets in terms of the Relative Pose Error for rotation part (\textdegree).}} The experimental results demonstrate that rolling shutter distortions affect the accuracy of motion trajectory estimations. Due to proper modeling, our method performs much better than state-of-the-art methods. It also demonstrates that cubic B-Spline interpolation is superior to linear interpolation. x denotes method failed on the corresponding sequence.}
%		\label{rpe_rot}
%		\vspace{-0.5em}
%		%	\setlength\tabcolsep{2pt}
%		\scriptsize
%		\setlength{\tabcolsep}{2.5mm}
%		\setlength{\belowcaptionskip}{-10pt}
%		\resizebox{\linewidth}{!}{
%			\begin{tabular}{c|c c c c c c}
%				\toprule
%				\makebox[0.08\textwidth][c]{} & \makebox[0.08\textwidth][c]{\scriptsize COLMAP} & \makebox[0.08\textwidth][c]{\scriptsize BARF} & \makebox[0.08\textwidth][c]{\scriptsize RSBA} & \makebox[0.08\textwidth][c]{\scriptsize NW-RSBA} & \makebox[0.08\textwidth][c]{\scriptsize USB-NeRF-linear} &\makebox[0.08\textwidth][c]{\scriptsize USB-NeRF-cubic} \\
%				%			&{\scriptsize \qquad COLMAP \qquad} &{\scriptsize BARF} &{\scriptsize \qquad RSBA \qquad} & {\scriptsize NW-RSBA} & {\scriptsize \qquad USB-NeRF-linear \qquad} & {\scriptsize \qquad USB-NeRF-cubic \qquad} \\
%				\midrule
%				Carla 		&2.357 $\pm$ 1.647 & 2.762 $\pm$ 2.041 & 1.844 $\pm$ 1.080 & 2.090 $\pm$ 1.492 & 0.586 $\pm$ 0.174 & \bf 0.528 $\pm$ 0.157 \\
%				
%				BlueRoom & 2.594 $\pm$ 1.411 & 8.123 $\pm$ 3.585 & 7.257 $\pm$ 3.413 & x            & 0.127 $\pm$ 0.074 & \bf 0.046 $\pm$ 0.041 \\
%				LivingRoom & 2.145 $\pm$ 1.320 & 9.016 $\pm$ 6.243 & 7.405 $\pm$ 4.383 & x            & 0.381 $\pm$ 0.140 & \bf 0.108 $\pm$ 0.053 \\
%				WhiteRoom & 1.810 $\pm$ 0.771 & 4.702 $\pm$ 2.077 & 4.212 $\pm$ 1.631 & x            & 0.194 $\pm$ 0.127 & \bf 0.089 $\pm$ 0.039 \\
%				
%				Adornment & 2.723 $\pm$ 1.438 & 10.390 $\pm$ 4.659 &       x     & x            & 0.581 $\pm$ 1.273 & \bf 0.234 $\pm$ 0.147 \\
%				Factory & 2.194 $\pm$ 1.187 & 8.523 $\pm$ 4.028 &        x     & x            & 0.209 $\pm$ 0.112 & \bf 0.135 $\pm$ 0.080 \\
%				Tanabata & 2.744 $\pm$ 1.662 & 15.187 $\pm$ 13.197 &        x     & x            & 1.042 $\pm$ 0.459 & \bf 1.008 $\pm$ 0.463 \\
%				
%				\midrule
%				
%				Avg. & 2.367$\pm$ 1.348 & 8.386$\pm$ 5.119 & 5.179$\pm$ 2.627 & 2.090$\pm$ 1.492 & 0.446$\pm$ 0.337 & \bf 0.307$\pm$ 0.140 \\
%				
%				\bottomrule
%			\end{tabular}
%		}
%	\end{center}
%\end{table}
%
%
%\begin{table}[t]
%	\begin{center}
%		\vspace{-1em}
%		\captionsetup {font={small,stretch=0.5}}
%		\caption{{\textbf{Quantitative comparisons on real datasets in terms of the Relative Pose Error for rotation part (\textdegree).}} The experimental results demonstrate that rolling shutter distortions affect the accuracy of motion trajectory estimations. Due to proper modeling, our method performs much better than state-of-the-art methods. It also demonstrates that cubic B-Spline interpolation is superior to linear interpolation. x denotes method failed on the corresponding sequence.}
%		\label{rpe_rot}
%		\vspace{-0.5em}
%		%	\setlength\tabcolsep{2pt}
%		\scriptsize
%		\setlength{\tabcolsep}{2.5mm}
%		\setlength{\belowcaptionskip}{-10pt}
%		\resizebox{\linewidth}{!}{
%			\begin{tabular}{c|c c c c c c}
%				\toprule
%				\makebox[0.08\textwidth][c]{} & \makebox[0.08\textwidth][c]{\scriptsize COLMAP} & \makebox[0.08\textwidth][c]{\scriptsize BARF} & \makebox[0.08\textwidth][c]{\scriptsize RSBA} & \makebox[0.08\textwidth][c]{\scriptsize NW-RSBA} & \makebox[0.08\textwidth][c]{\scriptsize USB-NeRF-linear} &\makebox[0.08\textwidth][c]{\scriptsize USB-NeRF-cubic} \\
%				%			&{\scriptsize \qquad COLMAP \qquad} &{\scriptsize BARF} &{\scriptsize \qquad RSBA \qquad} & {\scriptsize NW-RSBA} & {\scriptsize \qquad USB-NeRF-linear \qquad} & {\scriptsize \qquad USB-NeRF-cubic \qquad} \\
%				\midrule
%				seq1  & 0.278 $\pm$ 0.284 & 0.283 $\pm$ 0.152 & 0.578 $\pm$ 0.470 & 0.671 $\pm$ 0.545 & 0.114 $\pm$ 0.072 & \bf 0.108 $\pm$ 0.071 \\
%				seq2  & 0.794 $\pm$ 0.428 & \bf 0.737 $\pm$ 0.432 & 9.789 $\pm$ 14.344 & 28.325 $\pm$ 40.662 & 1.365 $\pm$ 1.733 & 0.777 $\pm$ 0.838 \\
%				seq3  & 0.271 $\pm$ 0.145 & 0.272 $\pm$ 0.176 & 0.397 $\pm$ 0.208 & 0.250 $\pm$ 0.116 & 0.159 $\pm$ 0.115 & \bf 0.145 $\pm$ 0.108 \\
%				seq4  & 0.225 $\pm$ 0.100 & 0.211 $\pm$ 0.110 & 0.247 $\pm$ 0.126 & 1.049 $\pm$ 0.571 & 0.160 $\pm$ 0.093 & \bf 0.155 $\pm$ 0.093 \\
%				seq5  & 0.607 $\pm$ 0.286 & 0.545 $\pm$ 0.199 & 2.245 $\pm$ 1.784 & 3.131 $\pm$ 2.316 & 0.168 $\pm$ 0.087 & \bf 0.166 $\pm$ 0.082 \\
%				seq6  & 0.345 $\pm$ 0.163 & 0.322 $\pm$ 0.247 & 0.575 $\pm$ 0.257 & 0.851 $\pm$ 0.874 & 0.180 $\pm$ 0.089 & \bf 0.149 $\pm$ 0.080 \\
%				seq7  & 0.219 $\pm$ 0.123 & 0.224 $\pm$ 0.143 & 0.324 $\pm$ 0.201 & 1.063 $\pm$ 0.700 & 0.146 $\pm$ 0.100 & \bf 0.128 $\pm$ 0.097 \\
%				seq8  & 0.520 $\pm$ 0.325 & 0.249 $\pm$ 0.103 & 0.502 $\pm$ 0.251 & 1.718 $\pm$ 1.011 & 0.151 $\pm$ 0.069 & \bf 0.135 $\pm$ 0.066 \\
%				seq9  & 0.322 $\pm$ 0.165 & 0.445 $\pm$ 0.276 & 4.400 $\pm$ 7.312 & 41.983 $\pm$ 47.732 & \bf 0.193 $\pm$ 0.211 & 0.263 $\pm$ 0.524 \\
%				seq10 & 0.351 $\pm$ 0.165 & 1.006 $\pm$ 2.460 & 1.889 $\pm$ 1.117 & 4.752 $\pm$ 4.748 & \bf 0.193 $\pm$ 0.277 & 0.250 $\pm$ 0.499 \\
%				
%				\midrule
%				Avg.   & 0.393 $\pm$ 0.218 & 0.429 $\pm$ 0.430 & 2.095 $\pm$ 2.607 & 8.379 $\pm$ 9.928 & 0.283 $\pm$ 0.285 & \bf 0.227 $\pm$ 0.246 \\
%				\bottomrule
%			\end{tabular}
%		}
%	\end{center}
%\end{table}
